# Supplementary material for: Deciphering High-order Structural Correlations within Fluxional Molecules from Classical and Quantum Configurational Entropy
Source: arXiv:2006.13624 ancillary file (2020-06-24)
Supplement: Supplementary file 1 [file TopolnickiBrieucSchranMarx_SupplementaryInformation.pdf]

# Supplementary Information

## Deciphering High-order Structural Correlations within Fluxional Molecules from Classical and Quantum Configurational Entropy


Rafał Topolnicki,[1,2] Fabien Brieuc,[1] Christoph Schran,[1,3] and Dominik Marx[1]

[1)] *Lehrstuhl für Theoretische Chemie, Ruhr-Universität Bochum, 44780 Bochum, Germany*

[2)] *Institute of Experimental Physics, University of Wrocław, 50-204 Wrocław, Poland*

[3)] *Present Address: Department of Physics and Astronomy, University College London, London, WC1E 6BT, UK*

CONTENTS

**I. High-dimensional Neural Network Potential Energy Surface** 3
A. Validation of NN-PES Energy Prediction 6
B. Validation of NN-PES Stationary Point Relative Energies 7
C. Validation of NN-PES Normal Mode Frequencies 8
D. Validation of NN-PES along Potential Energy Scans 9
E. Validation of NN-PES using MD and PIMD Simulations 10

**II. Quantum Simulations** 11
A. Validation of Path Integral Convergence: Trotter Discretization 11
B. Validation of Path Integral Convergence: Structures 12
C. Validation of Path Integral Convergence: Interaction Information 16

**III. Interaction Information Analyses** 17
A. Validation of Threshold Values for Structure Classification 17
B. Validation of Statistical Convergence of Interaction Information Estimator 19
C. Validation of $k$-Convergence of Interaction Information Estimator 21

**IV. Supplementary Data** 24
A. Analysis of All Interactions of Second Order 24
B. Analysis of All Interactions of Third and Fourth Order 26

**References** 27

# I. HIGH-DIMENSIONAL NEURAL NETWORK POTENTIAL ENERGY SURFACE

The high-dimensional neural network potential (HD-NNP) technique[1–4] was used to represent the global potential energy surface (PES) of the protonated acetylene molecule, $C_2H_3^+$, without reducing its dimensionality at the quality level given by CCSD(T*)-F12a/aug-cc-pVTZ electronic structure calculations (see below). In the HD-NNP approach, each atom type (meaning "nucleus corresponding to a chemical element", such as C and H in the present case) is associated with its own neural network (here: feedforward fully connected multi-layer perceptron) which takes as input the local environment around each atom of that type and outputs the associated atomic contribution to the potential energy. The final output is the total potential energy obtained by summing all atomic contributions of all types. The local atomic environment is described here using many–body atom–centered symmetry functions[5] ensuring a description that is invariant to translation and rotation of the whole molecule and to permutations of identical atoms.

In order to exhaustively sample the configuration space of the molecule effectively, which is needed to extract a set of structures used to fit (train, learn) the HD-NNP, and to keep the number of reference coupled cluster calculations as low as possible at the same time, we applied the automated fitting procedure as introduced recently by us[6] and reviewed in Ref. 7 to which we refer for full background and technical discussion, but it can be concisely summarized as follows. In the first step, a set of Born-Oppenheimer ab initio molecular dynamics (AIMD) simulations[8] using classical nuclei was performed for an isolated protonated acetylene molecule in vacuum at a set of temperatures from 1 K up to 1600 K using the `CP2k` simulation package.[9,10] At this initialization stage, the electronic structure of protonated acetylene was described based on density functional theory (DFT) using the local density approximation (LDA), DZVP basis set and Goedecker-Teter-Hutter pseudopotentials.[11]

Based on these trajectories, a very small number of structures was randomly extracted from this ensemble of configurations and reference calculations of the associated total (i.e. potential) energy was performed using coupled cluster theory (see below for details) to describe the electronic structure instead of DFT. This first small set of data points is then used to fit two distinct NNPs, both having the same architecture but being initialized with different random weights.

In the next step, both NNPs are used to predict the potential energy for all original DFT structures. These energy calculations are very inexpensive since NNPs are used and, therefore, they can be carried out easily using all structures that have been generated during the original AIMD simulations. Afterwards, very few configurations for which the energies predicted by the two NNPs differs the most are selected (as few as 20 in this case). The potential energy for these most-ill-predicted configurations is calculated using the reference method, i.e. the very same coupled cluster method as before, and the configurations are then added to the data set for fitting. After that, the procedure starts over again by fitting two NNPs based on the just extended reference data set of coupled cluster quality.

This procedure allows for the selection of the most representative points in the starting ensemble of configurations in an unbiased fashion while keeping the number of required expensive coupled cluster calculations as small as possible. Within this approach, the energy of the selected points is calculated with coupled cluster accuracy but the actual atom arrangements and thus the picked configurations were generated using DFT. The configurations present in the data set are thus biased with respect to those that would be given by the desired, but unknown, coupled cluster potential energy surface.

Finally, in order to sample on the coupled cluster PES itself, the boundaries of the NNP have to be improved by expanding the configuration space and lifting the bias. This is achieved by running a variety of classical MD and path integral MD (PIMD) simulations at different conditions (here temperatures) using the previously determined NNP. During these simulations, the first few configurations for which the NNP is extrapolating (meaning that values of the symmetry functions are outside the range corresponding to configurations which have been encountered before) are identified. These configurations lie outside of the data set used for training and the NNP is thus unable to give a reliable prediction of their energy. When several of these points have been recognized, the (MD or PIMD) simulations are aborted and the coupled cluster calculations are then performed for the identified extrapolating configurations to selectively and adaptively improve the data set by expanding its boundaries. As previously, configurations that feature the highest discrepancy between the energies predicted by two independent NNPs are also extracted from the these trajectories. This way, those regions of the training set that might not have been fully represented yet are systematically identified and improved using coupled cluster theory. Therefore not only the boundaries of the NNP are being expanded but also the NN-PES is

being successfully gauged away from what is obtained from DFT toward the desired coupled cluster reference method. The procedure described above is being repeated until the NNP is able to support long-time stable (i.e. non-extrapolating) MD and PIMD simulations under the desired conditions.

The particular neural network topology that we used to parameterized the NN-PES of protonated acetylene consists of two fully connected hidden layers, each containing 30 nodes activated by the hyperbolic tangent function, while the output layer consists of only one node activated by a linear function. The NNPs have been trained by first splitting the set of coupled cluster reference data into a training set which encompasses 90% of respective data points and a test set containing the remaining 10%; note that the latter data set is called "validation set" in some literature. Afterwards, the weights of the NNP have been optimized to minimize the error on the training set, while the error on the test test is monitored to avoid overfitting and to provide an estimate for the accuracy of the model on data that has never been seen.

The parameterization of the NN-PES for protonated acetylene (dubbed "V1-PES-Protonated-Acetylene-2020") has been performed using our in-house `RubNNet4MD` neural network package[12] as interfaced with the `CP2k` simulation package.[9,10] Therein, the adaptive element-decoupled extended Kalman filter[13–16] is implemented and has been utilized in the present case to optimize efficiently the weight parameters.

The coupled cluster reference calculations have been performed using the F12a explicitly correlated coupled cluster singles and doubles method with scaled perturbative triple corrections[17,18] in conjunction with Dunning's augmented correlation-consistent polarized valence triple-zeta basis set,[19] meaning CCSD(T*)-F12a/aug-cc-pVTZ theory and abbreviated by us in the following simply by CCSD(T*), as implemented in the `Molpro` package.[20] The triple-zeta basis in conjunction with the approximate F12a correlation factor has been shown to provide energies that are close to complete basis set (CBS) limit.[18]

The resulting global NN-PES for protonated acetylene of CCSD(T*) quality was thoroughly validated with respect to corresponding single-point coupled cluster calculations (contained neither in the training nor test sets used to fit and test the NN-PES) as shown in the subsequent subsections. In addition, we refer in the context of validation to the minimum energy isomerization pathway that connects the global bridged and local Y-shaped minima as depicted in Fig. 1 in the main text.

### A. Validation of NN-PES Energy Prediction

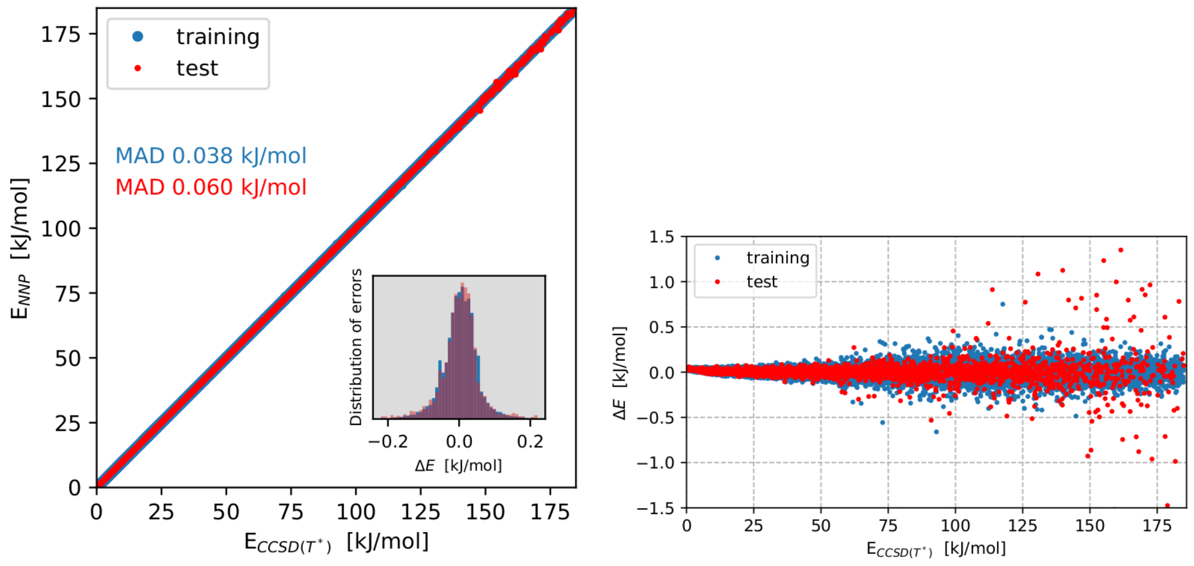


FIG. 1. Correlation of the potential energy obtained from explicit CCSD(T*) calculations and from the final NN-PES representation of protonated acetylene.

The correlation of the potential energy from explicit CCSD(T*) single-point calculations and from evaluating the final NN-PES used to perform all entropy analyses is presented in Fig. 1. Therein, the mean absolute difference is given separately for training (blue color) and test set (red color). The right panel shows the difference between CCSD(T*) reference calculations and the NN-PES predictions over the entire range of reference energies, while the histogram inset in the left panel presents its distribution around zero in the respective color.

This analysis shows that our NN-PES provides a rather uniform quality of energy predictions across a large part of the relevant configuration space of protonated acetylene, thus including low- and high-energy structures. Importantly, this NN-PES has not been designed to properly describe the different (closed- and open-shell) dissociation channels that can lead to fragmentation of protonated acetylene at very high temperatures (exceeding by far the highest one used in our present study). We note in passing that including dissociation would be possible at the level of the neural network technology by feeding configuration that have been systematically sampled from fragmentation trajectories into the set of reference

data. However, at the level of the underlying electronic structure method, this endeavor would necessarily call for using multireference coupled cluster methodology for well-known reasons.

## B. Validation of NN-PES Stationary Point Relative Energies

The performance of the NN-PES has also been gauged specifically with respect to encoding the correct relative energies of the relevant stationary points on the global PES which describes protonated acetylene, see Table I. One observes that the absolute errors of all

TABLE I. Energy differences (in kJ/mol) between the three relevant stationary points on the PES of protonated acetylene: Y-shaped versus bridged structure $\Delta E^{\mathrm{Y-B}}$, transition state versus bridged structure $\Delta E^{\mathrm{TS-B}}$, and transition state versus Y-shaped structure $\Delta E^{\mathrm{TS-Y}}$ computed using NN-PES and CCSD(T*), see Fig. 1 in the main text for these configurations. The energies of the Y-shaped and bridged configurations for both, NN-PES and CCSD(T*), were taken from individual respective geometry optimizations while the transition state configuration was obtained from the NEB path obtained from the NN-PES (as shown in Fig. 1 in the main text) based on which a CCSD(T*) single-point energy calculation has been performed.

| | $\Delta E^{\mathrm{Y-B}}$ | $\Delta E^{\mathrm{TS-B}}$ | $\Delta E^{\mathrm{TS-Y}}$ |
|---|---|---|---|
| CCSD(T*) | 15.9306 | 16.4597 | 0.5290 |
| NN-PES | 15.9631 | 16.4626 | 0.4995 |
| Error | 0.0325 | 0.0029 | −0.0296 |
| Error % | 0.2041 | 0.0179 | −5.5870 |

energy differences are of a similar magnitude, about 0.01 kJ/mol, which supports the earlier conclusion that this NN-PES provides a uniform quality across the relevant configuration space. Clearly, the corresponding relative error of the transition state energy relative to the Y-shaped structure, corresponding to decay out of the shallow local minimum toward to global bridged minimum structure, appears to be large at first glance. But one has to keep in mind the tiny height of that barrier, $\approx 0.5$ kJ/mol (corresponding to about 0.1 kcal/mol, 60 K, 40 cm$^{-1}$, or 0.005 eV), which is one order of magnitude below what is considered to be “chemical accuracy”, namely 1 kcal/mol.

Overall, we draw the conclusion that the NN-PES provides a faithful representation in particular of this set of important structures of protonated acetylene.

## C. Validation of NN-PES Normal Mode Frequencies

Normal modes computed for the fully optimized bridged and Y-shaped stationary points of protonated acetylene as obtained by using explicit CCSD(T*) calculations and evaluating the NN-PES are compiled in Table II at the level of the harmonic frequencies. In all cases the step size utilized for numerical differentiation of the energy to construct the Hessian matrix was set to 0.0001 Å.

TABLE II. Normal modes frequencies (in $cm^{-1}$) of protonated acetylene in its bridged and Y-shaped stationary-point structures computed using CCSD(T*) calculations and from the NN-PES. The mean absolute error (MAE) and mean absolute percentage error (MAPE) are reported as measures of the quality of the NN-PES.

| | | | | | | | | | | |
|---|---|---|---|---|---|---|---|---|---|---|
| bridge | CCSD(T*) | 598.58 | 618.25 | 763.84 | 917.01 | 1258.96 | 1940.33 | 2355.97 | 3269.49 | 3367.73 |
| | NN-PES | 602.96 | 622.26 | 766.44 | 916.79 | 1259.53 | 1945.32 | 2357.13 | 3268.86 | 3370.29 |
| | Error | 4.38 | 4.01 | 2.60 | −0.22 | 0.57 | 4.99 | 1.16 | −0.63 | 2.56 |
| | Error % | 0.73 | 0.65 | 0.34 | −0.02 | 0.05 | 0.26 | 0.05 | −0.02 | 0.08 |
| | MAE | 2.35 | | | | | | | | |
| | MAPE % | 0.24 | | | | | | | | |
| Y | CCSD(T*) | 165.59 | 633.20 | 814.97 | 1079.34 | 1169.93 | 1733.94 | 3006.06 | 3072.86 | 3288.41 |
| | NN-PES | 170.03 | 629.15 | 820.16 | 1076.02 | 1162.87 | 1733.08 | 3006.31 | 3082.20 | 3284.68 |
| | Error | 4.44 | −4.05 | 5.19 | −3.32 | −7.06 | −0.86 | 0.25 | 9.34 | −3.73 |
| | Error % | 2.68 | −0.64 | 0.64 | −0.31 | −0.60 | −0.05 | 0.01 | 0.30 | −0.11 |
| | MAE | 4.25 | | | | | | | | |
| | MAPE % | 0.59 | | | | | | | | |

On average, the harmonic frequencies obtained by evaluating the NN-PES are seen to deviate from those obtained from explicit CCSD(T*) reference calculations by roughly half a percent only.

## D. Validation of NN-PES along Potential Energy Scans

To further test the accuracy of the neural network potential we computed additional potential energy scans which were compared with CCSD(T*) results in Fig. 2. The bare eye cannot notice significant deviations of the NN-PES fit from the dense points obtained from explicit CCSD(T*) calculations except for the panel in the center. This, however, corresponds to the ideal orbiting motion of the equatorial proton around the basically collinear H–C–C–H axis of the bridged global minimum of protonated acetylene, which is a close to barrierless pathway with an essentially vanishing energy barrier of 0.06 kJ/mol.

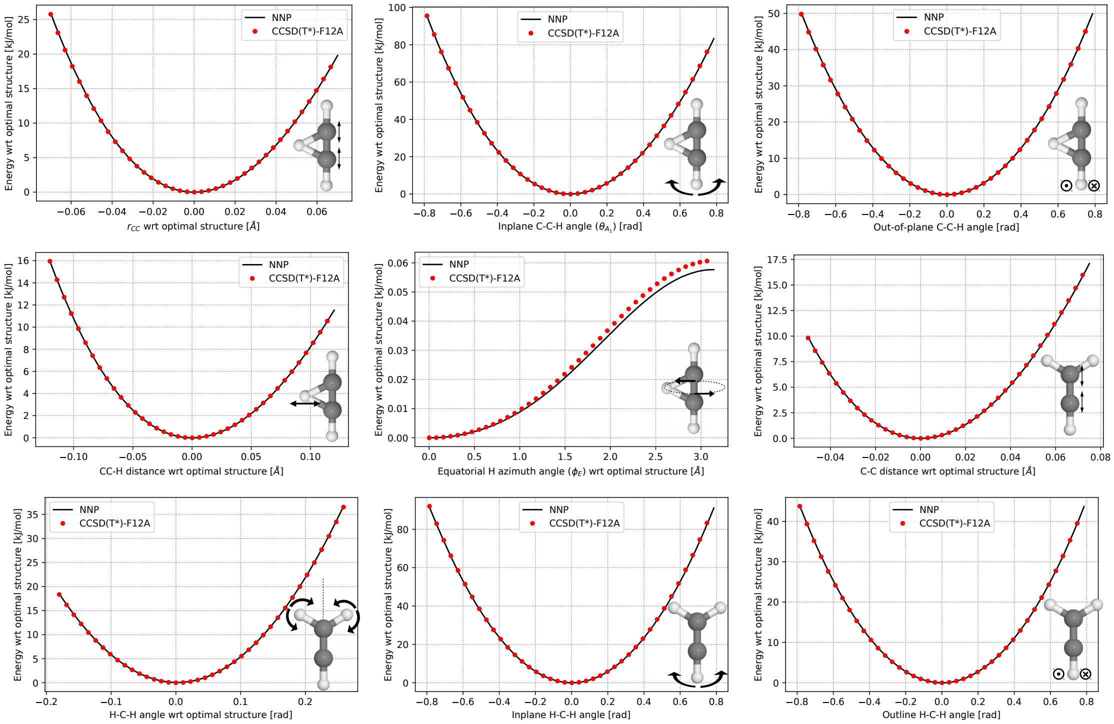


FIG. 2. Selected potential energy scans computed using explicit CCSD(T*) single-point calculations (red dots) and by evaluating the NN-PES (black solid lines) with reference to the bridged and Y-shaped minimum energy structures of protonated acetylene as indicated by the insets. Each plot is accompanied by a structural model with arrows that visualized the considered distortion of the minimum energy structure. Note that the energy scale is adjusted in each panel as to properly cover the respective minimum and maximum energies along that path.

Overall, we find that the NN-PES very accurately and also faithfully represents the global energy landscape of protonated acetylene even when moving quite far away from the relevant minima (while not considering any dissociation channel as explained before).

## E. Validation of NN-PES using MD and PIMD Simulations

Last but not least, the NN-PES was validated based on a subset of the molecular dynamics production runs that we used for the interaction information analyses. To this end, MD simulations at 300, 800, 1200 and 1600 K as well as PIMD simulations at 2, 5, 25 K were used to randomly sample 100 points from the last 250 ps of each trajectory and re-evaluated using single-point CCSD(T*) reference calculations. This provides us with a realistic test set consisting of additional 700 configurations in total. In all cases the mean absolute difference between NNP and reference calculations does not exceed the one obtained during training as supported by these data presented in Fig. 3.

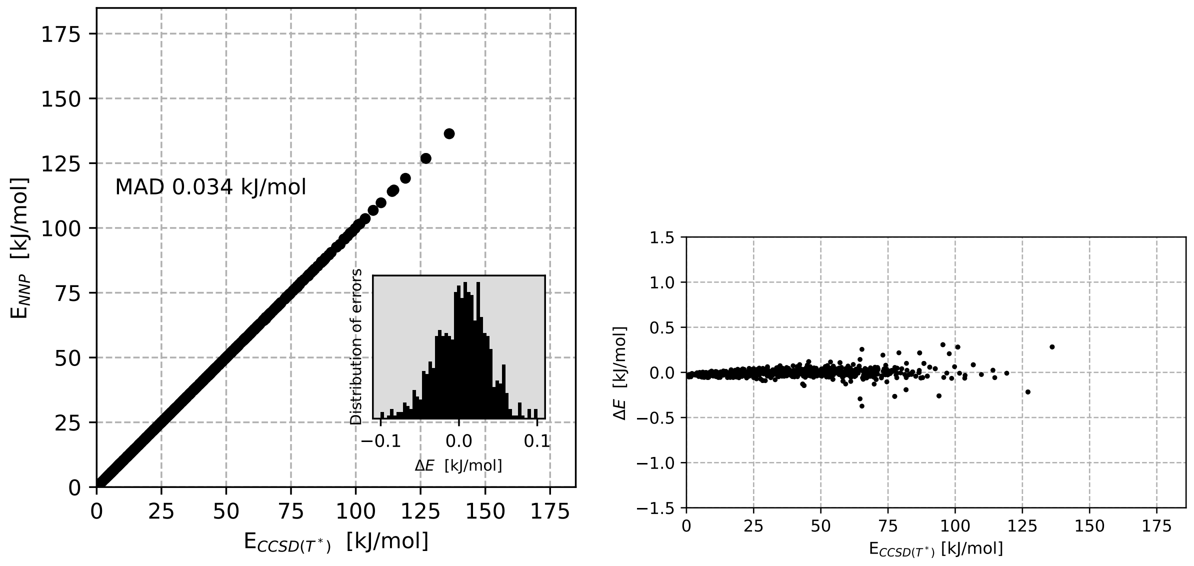


FIG. 3. Correlation of the NN-PES potential energies for a random sample of configurations (as encountered along the MD and PIMD trajectories used to actually carrying out the interaction information analysis, see text) and explicit CCSD(T*) single-point calculations performed the same configurations; cf. discussion of Fig. 1 for such comparisons.

This uncompromised reality check proves that the generated NN-PES enables us to perform in practice both, classical MD and quantum PIMD simulations of protonated acetylene at CCSD(T*) accuracy.

## II. QUANTUM SIMULATIONS

In the context of the simulations underlying this study, we refer the reader to a recent review article[7] that unfolds the entire methodological framework that allows us to carry out converged quantum simulations of fluxional molecules or complexes even at cryochemical conditions. In what follows, we scrutinize the level of path integral discretization that is required to carry out converged PIMD simulations all the way from 1600 K, where protonated acetylene can be accurately described even when using classical MD, down to 1 K where carefully discretized quantum PIMD simulations are called for.

As comprehensively reviewed recently,[7] PIMD simulations can be performed efficiently when using the so-called PIQTB thermostat[21] as implemented by us in `CP2k` to converge the path integral in terms of its discretization in terms of the number of Trotter relica $P$ (or beads or imaginary time slices) even at cyrogenic temperatures.[22] In order to gauge convergence of the PIQTB method, the standard so-called PILE thermostat[23] can be used at the expense of using much larger $P$ values in the end to ultimately achieve convergence. These techniques are applied in the following subsections to protonated acetylene in order to compute relevant observables, not only considering structural distribution functions but in particular also all significant $n$-coordinate interactions informations $I_n$ up to the four-body terms.

### A. Validation of Path Integral Convergence: Trotter Discretization

The first quantity to check convergence for are the radii of gyration of all nuclei within protonated acetylene. They are a measure of the spatial extent or delocalization of the nuclei due to quantum fluctuations at a given temperature, quantify the amplitude of zero-point vibrational motion in the quantum ground state, and vanish identically for classical point particles at any temperature. For PIQTB thermostat together with $P = 48$ replica is sufficient to provide convergence of these properties at $T = 100$ K according to the data

shown in Fig. 4; note the logarithmic scale of the $P$ axis. The number of replicas $P$ used for the simulations at different temperatures was determined as usual in such a way that the product $P \cdot T$ remains constant at all temperatures, which is expected to provide similar Trotter accuracy independently from temperature. We make the reader aware that this level of convergence requires us to use 4 800 replica at the lowest temperature considered in the present study being 1 K.

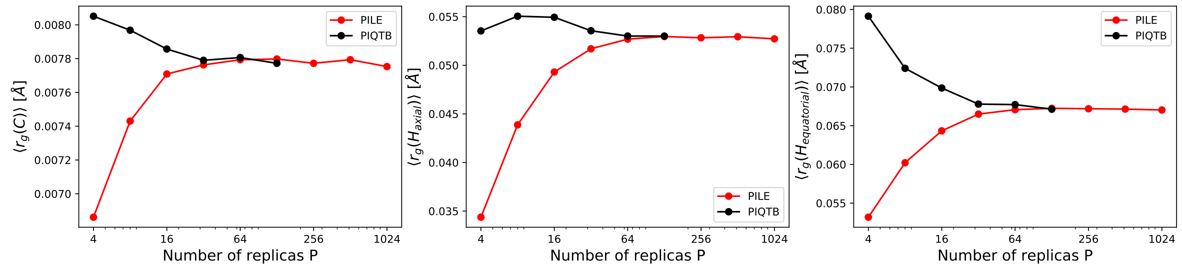


FIG. 4. Radii of gyration $\langle r_{\rm g} \rangle$ of the carbon (left), axial hydrogen (middle), and equatorial hydrogen (right) nuclei at 100 K as a function of the number of Trotter replica $P$ for protonated acetylene obtained using the PIQTB (red lines) and PILE (black lines) thermostats, see text, in conjunction with the PIMD simulations based on the NN-PES.

## B. Validation of Path Integral Convergence: Structures

Moving from quantum effects at the level of nuclear delocalization to their impact on molecular structure, we present now the quantum probability distributions functions involving the C–H and H–H distances as well as the H–C–C angle within protonated acetylene in Figs. 5, 6 and 7, respectively.

This analysis confirms that our discretization product for PIQTB simulations leading to $P = 4\,800/T$ as determined to converge the delocalization of the nuclei in space suffices to also converge the molecular structure of protonated acetylene. Importantly, this is also true at 5 K, which is the lowest temperature for which we could converge the simulation using standard PILE thermostatting within PIMD in view of the enormous Trotter discretization required, namely $P = 4\,096$, whereas $P = 20\,480$ for using PILE at 1 K would be very demanding. Recall, however, that the PIQTB quantum simulations at 1 K have been carried out using the required discretization of $P = 4\,800$ converges the path integral.

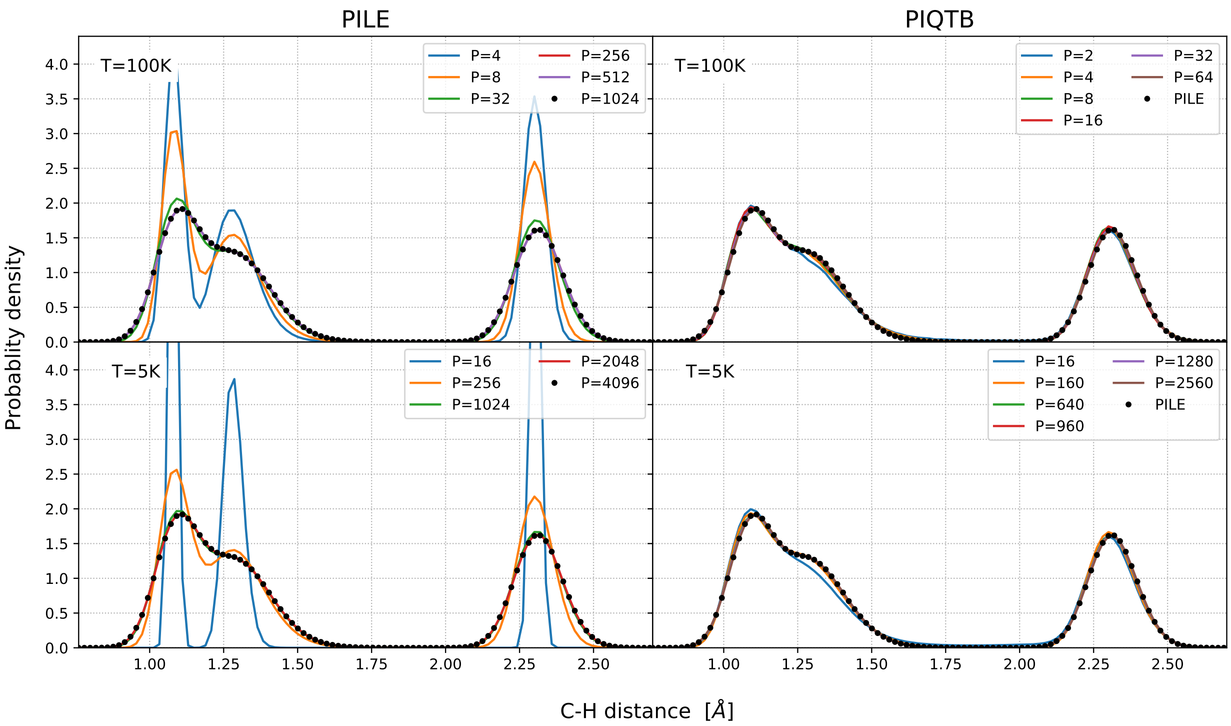


FIG. 5. Quantum distribution functions of the carbon-hydrogen distance for different numbers of replicas $P$ at $T = 100$ and $5\,\mathrm{K}$ using PILE (left) and PIQTB (right) thermostats within PIMD. The dashed black lines in the right panels correspond to the PILE data obtained with the largest considered $P$ value in the corresponding left panel.

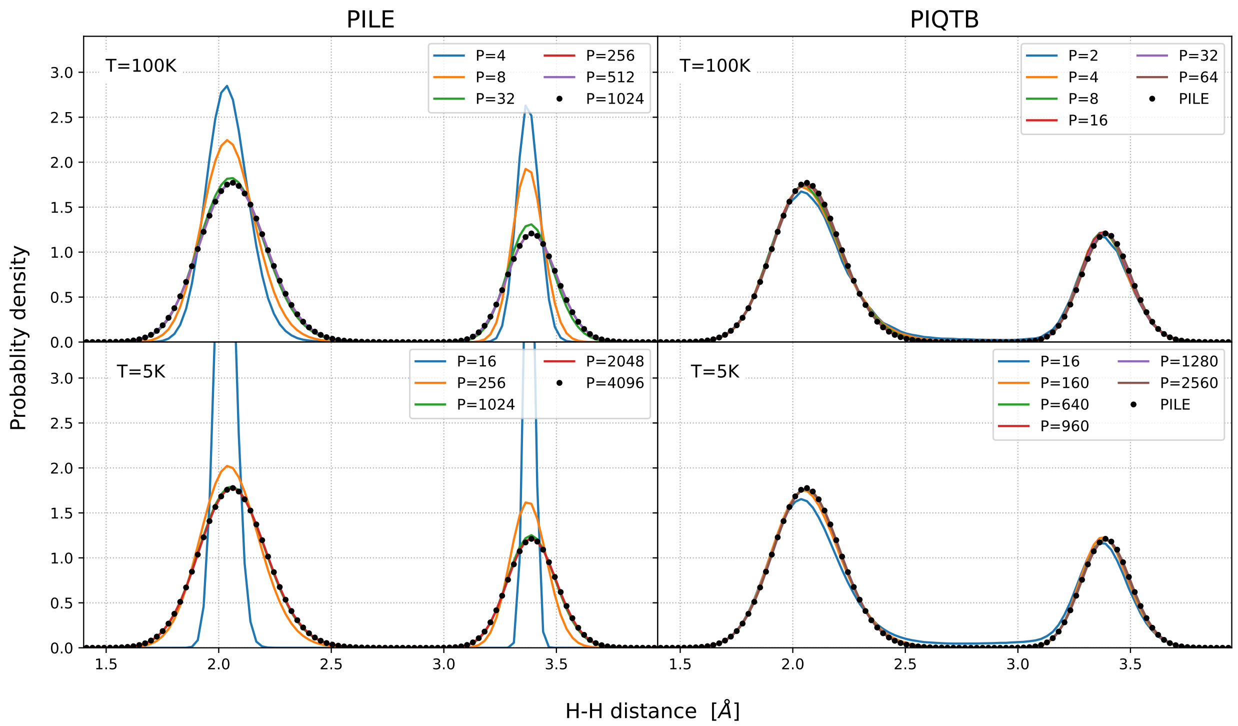


FIG. 6. Quantum distribution functions of the hydrogen-hydrogen distance for different numbers of replicas $P$ at $T = 100$ and $5\,\mathrm{K}$ using PILE (left) and PIQTB (right) thermostats within PIMD. The dashed black lines in the right panels correspond to the PILE data obtained with the largest considered $P$ value in the corresponding left panel.

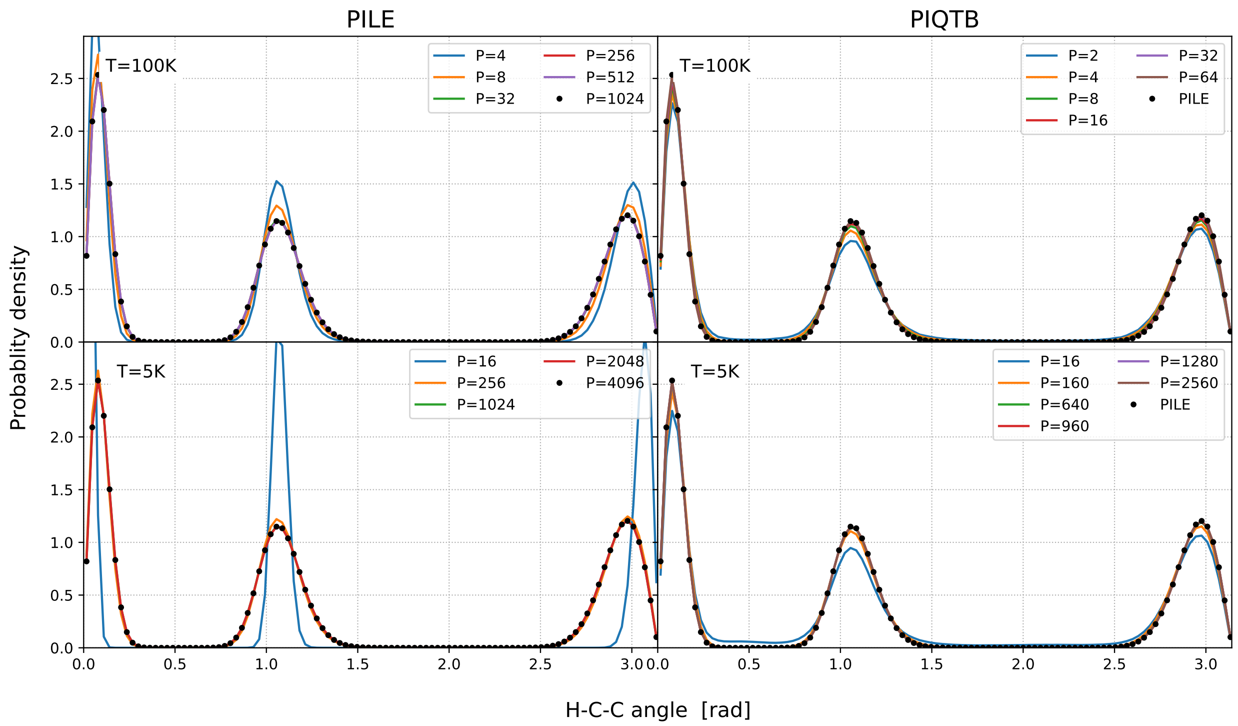


FIG. 7. Quantum distribution functions of the hydrogen-carbon-carbon angle $\angle_{HCC}$ for different numbers of replicas $P$ at $T = 100$ and $5\,\mathrm{K}$ using PILE (left) and PIQTB (right) thermostats within PIMD. The dashed black lines in the right panels correspond to the PILE data obtained with the largest considered $P$ value in the corresponding left panel.

## C. Validation of Path Integral Convergence: Interaction Information

Finally, we also validate that our PIQTB quantum simulations using $P = 4\,800/T$ for all temperatures provide converged estimates of the $n$-coordinate interaction information which is the core property investigated in the main text. Thus, we compile in Fig. 8 all important correlations computed based on PILE and PIQTB simulations; note that the could no continue to use PILE at temperatures lower than 50 K due to the increasingly large Trotter discretization that would be required to converge the path integral as shown in the previous two subsections. An almost perfect match between the two methods is observed throughout. Only very small differences occur in case of the four-coordinate correlation $I_4(\theta_{\mathrm{E}}, \phi_{\mathrm{A}_1}, \phi_{\mathrm{A}_2}, \phi_{\mathrm{E}})$, yet the shape of the curve is preserved. Moreover, such high-order correlations require many more data points in the statistical sample to converge which allows us to speculate, factoring in all other very favorable comparisons, that PIQTB and PILE data also for $I_4$ would closely agree if longer PIMD trajectories were available.

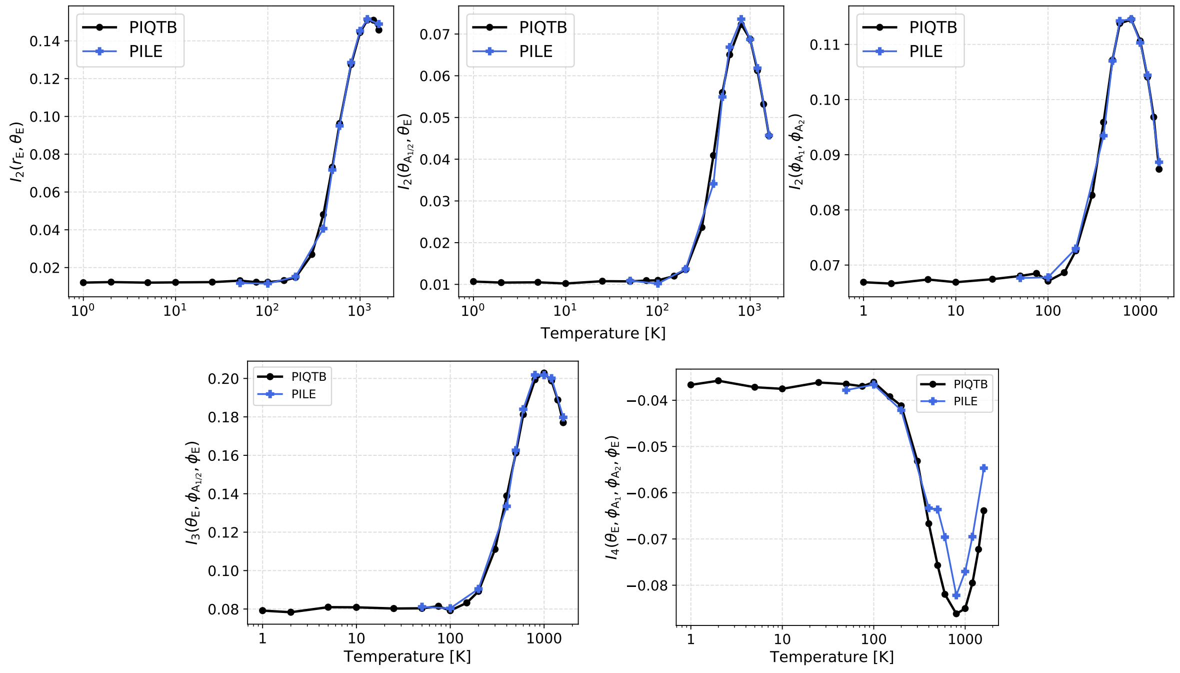


FIG. 8. All relevant $n =$ two-, three- and four-coordinate correlations $I_n$ of protonated acetylene as a function of temperature using PIQTB (black lines) and PILE (blue lines) thermostats within PIMD; the Trotter discretization $P$ at each temperature is determined as described in the previous two subsections.

## III. INTERACTION INFORMATION ANALYSES

### A. Validation of Threshold Values for Structure Classification

As amply discussed in the main text, we have to classify each and every configuration of protonated acetylene for which we compute the interaction information as being bridge-like or not within our generalized coordinate system as defined with the help of Fig. 2 in the main text. A given structure is classified to be bridge-like based on considering the polar

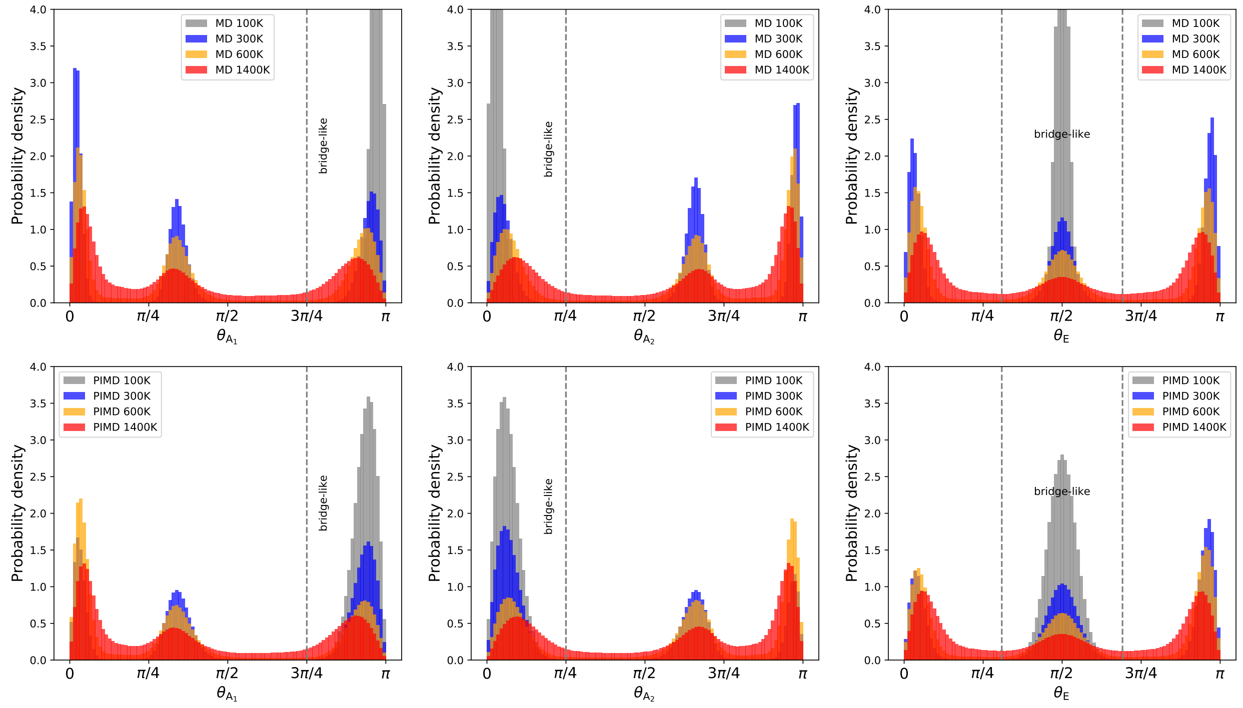


FIG. 9. Classical (top) and quantum (bottom) distribution functions of the polar angles of the two axial protons ($\theta_{A_1}, \theta_{A_2}$) and the equatorial proton ($\theta_E$) when permutations are not imposed as obtained from MD and PIMD simulations of protonated acetylene at the temperatures indicated within the panels. The vertical dashed lines mark the respective separatrices for bridge-like structures using the structure-based criteria (1) introduced in the text. Note that histogram bars corresponding to 100 K in the top panels extend beyond what is shown.

angles of all three protons, $\theta_{A_1}, \theta_{A_2}$ and $\theta_E$, where all possible respective permutations of the three H and two C atoms (i.e. nuclei) need to be taken into account to assure permutational invariance of the result. A sampled configuration is considered to be bridge-like if

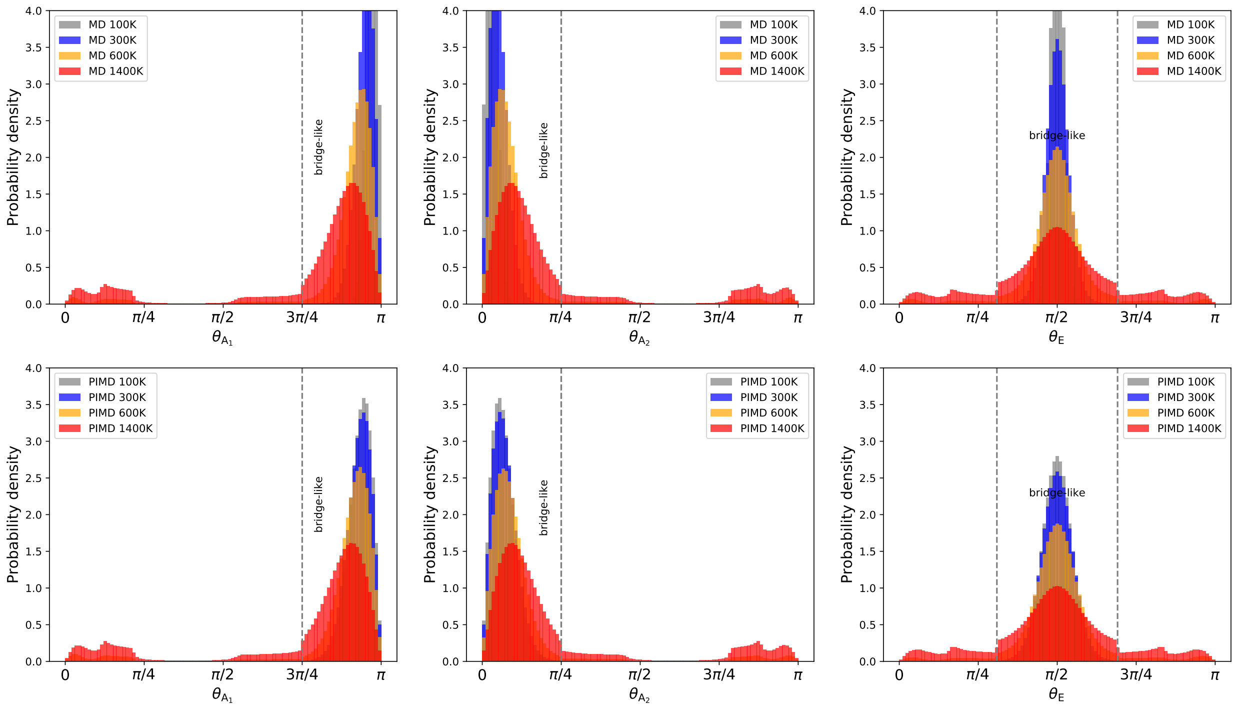


FIG. 10. Same as Fig 9 after considering the C and H permutations as explained in the text.

all three permutationally invariant angles are within certain bounds. These bounds can be determined from the simulations themselves when considering the three respective distribution functions as depicted in Fig. 9. As one can clearly see, these periodic probabilities feature minima that separate prominent maxima, the latter corresponding to close-to-ideal bridge configurations of protonated acetylene. Moreover, these minima are identical both, for classical and quantum simulations and upon varying the temperature. Thus, based on corresponding classical and quantum probability distribution functions in Fig. 9 we arrive at the following values for the windows within which we consider a random configuration to be bridge-like, namely

$$3\pi/4 \leq \theta_{\mathrm{A}_1} \leq \pi, \;\; 0 \leq \theta_{\mathrm{A}_2} \leq \pi/4 \;\; \text{and} \;\pi/2 - 0.6 \leq \theta_{\mathrm{E}} \leq \pi/2 + 0.6. \tag{1}$$

These criteria are applied throughout when computing the interaction informations $I_n$ of protonated acetylene as reported within this investigation.

Mind that the distribution functions presented in Fig. 9 were computed directly from the molecular dynamics structures and, thus, the C and H permutations were not taken into account. Therefore, most of the many structures that are not recognized as bridge-like are

identified to be in fact bridge-like once the permutations are properly imposed a posteriori. This is demonstrated by Fig. 10 which now presents the distributions of polar angles $\theta_{A_1}, \theta_{A_2}$ and $\theta_E$ when all possible permutations of C and H atoms are considered while each structure is considered only once: If for one of the permutations the conditions (1) are satisfied, then that given configuration is considered as bridge-like and only that permutation is taken into account to compute the polar angles. Otherwise, those values of polar angles are reported for the structure as they are encountered during the molecular dynamics run (i.e. without imposing a posteriori permutations).

Applying the structure-based criteria (1) to detect bridge-like configurations, we find that 99.99 % and 73 % of all configurations are found to be bridge-like at 100 K and 1400 K, respectively, in both quantum PIMD and classical MD simulations; note that the difference to 100 % does not indicate the relative contribution of Y-like structures though. This is consistent with the fact that the local minimum corresponding to Y-like structures is utmost shallow and, moreover, that the barrier to reach Y-like from bridge-like structures is quite high as reported in Table I. Together, this means that bridge-like structures of protonated acetylene are overwhelmingly populated in the canonical ensemble even up to high temperatures.

## B. Validation of Statistical Convergence of Interaction Information Estimator

Figure 11 depicts the estimated values of relevant two- and three-coordinate interaction informations, $I_2(r_E, \theta_E)$, $I_2(\phi_{A_1}, \phi_{A_2})$ and $I_3(\theta_E, \phi_{A_1}, \phi_E)$, as function of data set size, i.e. as function of the number of protonated acetylene configurations that have been sampled using MD and PIMD at representative temperatures in order to compute $I_n$. The dotted lines provide the boundaries for the region in which the estimated interaction information deviates from value obtained when using the maximum number of data points (i.e. approximately 25 million configurations) by less than 1 %. As can be seen, taking only 2 million points is in most cases already sufficient to provide results in the $\pm 1$ % statistical error range (as judged with respect to using all 25 million structures). Higher-order correlations generally requires more data points as is generally known.

All data sets considered in this study for analysis consisted of at least of 10 million protonated acetylene structures sampled from MD or PIMD simulations using the NN-PES which,

based on the present assessment, assures sufficient convergence of the reported interaction informations $I_n$.

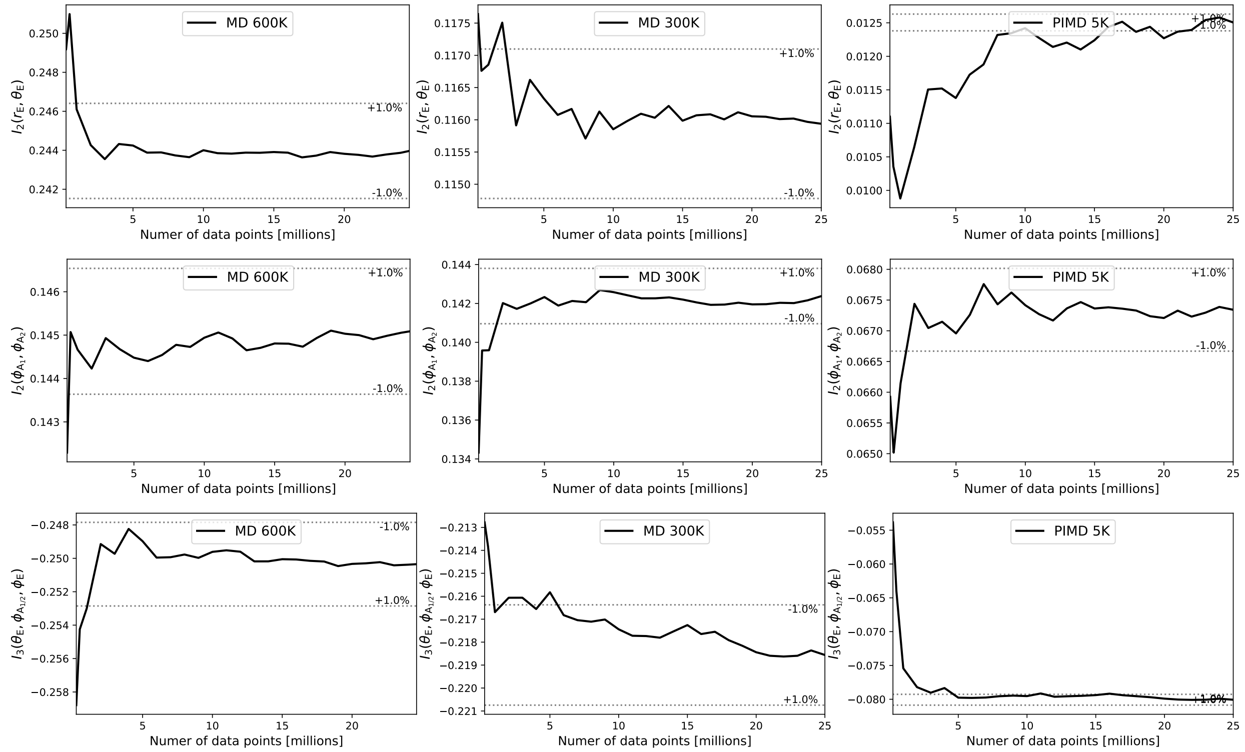


FIG. 11. Convergence of the interactions information estimators $I_2(r_\mathrm{E}, \theta_\mathrm{E})$, $I_2(\phi_{\mathrm{A}_1}, \phi_{\mathrm{A}_2})$ and $I_3(\theta_\mathrm{E}, \phi_{\mathrm{A}_{1/2}}, \phi_\mathrm{E})$ computed for protonated acetylene as a function of the statistical sample size as given by the number of data points (i.e. configurations reported in millions) used to compute $I_n$ based on $k = 5$ to compute the underlying $k$-NN entropy estimator. Classical MD and quantum PIMD simulations are used to generate the samples at the temperatures as provided in the panels. Two upper and lower horizontal dotted lines provide information about the variability of the estimate within $+1$ % and $-1$ %, respectively, compared to the estimate obtained when using the full data set of about 25 million structures in each case. Note that the vertical scale is adjusted in each panel as to properly cover the respective minimum and maximum $I_n$ values encountered.

## C. Validation of $k$-Convergence of Interaction Information Estimator

In order to the derive equation for the $k$-NN entropy estimator which we use, i.e.

$$S_k^{(N)} = \frac{1}{N}\sum_{i=1}^{N} \ln R_{i,k} + \ln \frac{N\pi^{s/2}}{\Gamma(\frac{s}{2}+1)} - L_{k-1} + \gamma \ , \tag{2}$$

from the definition of the configurational entropy

$$S(1,2,\ldots,s) = -\int f(\mathbf{q}) \ \ln f(\mathbf{q}) \, d\mathbf{q},$$

it is assumed that the underlying probability density $f$ can be approximated by a step function which is constant in the region of $k$ nearest neighbors around each sample point.[24,25] This assumption is better fulfilled for small values of $k$, therefore it is widely accepted to use $k = 1, \ldots, 5$ for instance,[26,27] providing a small systematic error (bias). At the same time, small values of the parameter $k$ translate into a greater variance of the entropy estimator given by Eq. (2). Thus, there obviously is a bias versus variance trade-off. Since the true value of entropy, hence also interaction information, is unknown in any practical application of the formalism, we are not able to choose the optimal value of $k$ based on minimization of the mean-square error. Instead we approximate the variance of interaction information estimators based on using the bootstrap procedure.[28] Bootstrapping allows one to assign measures of accuracy, such as the variance, to sample estimates using a resampling technique.

Figure 12 shows the relationship between the approximated values of the variance of the three representative interaction information estimators $I_2(r_\mathrm{E}, \theta_\mathrm{E})$, $I_2(\phi_{\mathrm{A}_1}, \phi_{\mathrm{A}_2})$ and $I_3(\theta_\mathrm{E}, \phi_{\mathrm{A}_{1/2}}, \phi_\mathrm{E})$ and the value of the parameter $k$ for MD and PIMD simulations. We can see that there is a very rapid decrease of variance for small values of $k$ which then becomes relatively constant for $k > 50$. For this assessment, we only used $10^6$ data points to estimate the underlying entropies and for larger data sets the plateau is expected to shift towards larger values of $k$. It is reasonable not to use the lowest possible value of $k$ as the obtained estimate will be prone to stochastic fluctuations. Since the estimated value of the bias is unknown, we propose here to use a rather small value of $k = 5$ in order to benefit from the rapid decay of the variance without introducing a significant systematic error.

In order to validate our choice we have considered values of $k$ up to 50 and also explicitly gauged the four-coordinate correlation $I_4$ for all temperatures using both, classical MD and quantum PIMD simulations of protonated acetylene. The data collected in Fig. 13

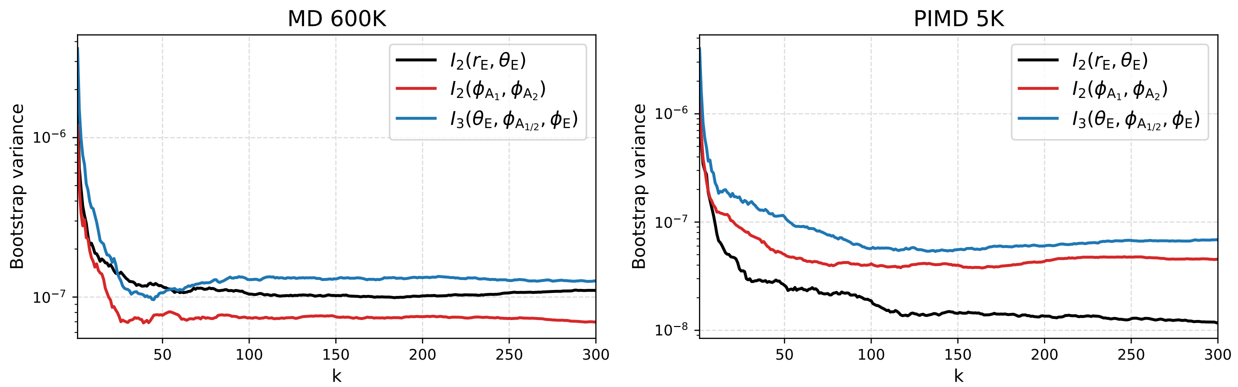


FIG. 12. Estimated values of standard deviation of three interaction information estimators $I_n$ as function of the parameter $k$ using 50 bootstrap repetitions while the number of data points (i.e. protonated acetylene configurations)used to compute the $k$-NN entropy estimators themselves was fixed to be $10^6$. Two representative simulations setups have been used for this assessment: classical MD at 600 K (left panel) and quantum PIMD at 5 K (right panel).

demonstrate that virtually no quantitative difference is observed. Moreover, the estimates obtained for $k = 2$ and 5 do not differ much, the only difference being that the first one producing more noisy estimates. Even when taking large values such as $k = 50$ we still get quantitatively the same results as for $k = 5$, see Fig. 13, which is a consequence of using very large data sets for our analysis, i.e. many protonated acetylene configurations sampled from MD and PIMD using the NN-PES.

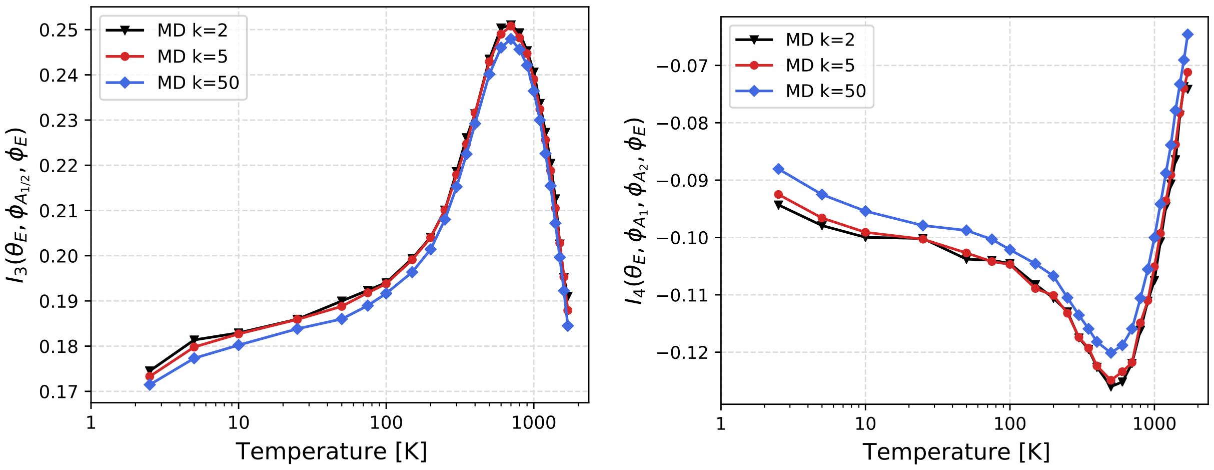


FIG. 13. Three- and four-coordinate correlations as a function of temperature for $k = 2$, 5 and 50, see text, obtained for protonated acetylene based on classical MD simulations. Corresponding plots based on quantum PIMD simulations provide the same kind of information and are thus not shown.

## IV. SUPPLEMENTARY DATA

### A. Analysis of All Interactions of Second Order

Only three types of two-coordinate and one type of three- and four-coordinate correlations are reported in the main text. Below we justify this approach by showing that all other correlations are negligible. We have found that the relative importance of the correlations neither depends on the temperature nor on treating the nuclei as classical or quantum point particles. The result of this analysis is presented in the following for two representative cases, namely for the classical description of the nuclei at 600 K and for the corresponding quantum treatment at 5 K.

Based on the data compiled in Tables III and IV it is clear that all two-body correlations other than those studied in the main text are many times weaker and thus negligible for the present discussion.

TABLE III. Interaction information matrix (dimensionless) involving all 10 generalized coordinates obtained from classical MD simulation at $T = 600\,\mathrm{K}$. The strongest correlations, hence those studied in detail in the main text, are typeset in bold.

| | $r_{\mathrm{CC}}$ | $r_{\mathrm{A}_1}$ | $\theta_{\mathrm{A}_1}$ | $r_{\mathrm{A}_2}$ | $\theta_{\mathrm{A}_2}$ | $r_{\mathrm{E}}$ | $\theta_{\mathrm{E}}$ | $\phi_{\mathrm{A}_1}$ | $\phi_{\mathrm{A}_2}$ | $\phi_{\mathrm{E}}$ |
|---|---|---|---|---|---|---|---|---|---|---|
| $r_{\mathrm{CC}}$ | – | 0.000 | 0.011 | 0.000 | 0.011 | 0.009 | 0.017 | 0.000 | 0.000 | 0.000 |
| $r_{\mathrm{A}_1}$ | | – | 0.000 | 0.000 | 0.000 | 0.000 | 0.001 | 0.000 | 0.000 | 0.000 |
| $\theta_{\mathrm{A}_1}$ | | | – | 0.000 | 0.008 | 0.035 | **0.104** | 0.000 | 0.000 | 0.000 |
| $r_{\mathrm{A}_2}$ | | | | – | 0.000 | 0.000 | 0.000 | 0.000 | 0.000 | 0.000 |
| $\theta_{\mathrm{A}_2}$ | | | | | – | 0.035 | **0.104** | 0.000 | 0.000 | 0.000 |
| $r_{\mathrm{E}}$ | | | | | | – | **0.243** | 0.000 | 0.000 | 0.000 |
| $\theta_{\mathrm{E}}$ | | | | | | | – | 0.000 | 0.000 | 0.000 |
| $\phi_{\mathrm{A}_1}$ | | | | | | | | – | **0.145** | 0.002 |
| $\phi_{\mathrm{A}_2}$ | | | | | | | | | – | 0.002 |
| $\phi_{\mathrm{E}}$ | | | | | | | | | | – |

TABLE IV. Interaction information matrix (dimensionless) involving all 10 generalized coordinates obtained from quantum PIMD simulation at $T = 5\,\mathrm{K}$. The strongest correlations, hence those studied in detail in the main text, are typeset in bold.

| | $r_{\mathrm{CC}}$ | $r_{\mathrm{A}_1}$ | $\theta_{\mathrm{A}_1}$ | $r_{\mathrm{A}_2}$ | $\theta_{\mathrm{A}_2}$ | $r_{\mathrm{E}}$ | $\theta_{\mathrm{E}}$ | $\phi_{\mathrm{A}_1}$ | $\phi_{\mathrm{A}_2}$ | $\phi_{\mathrm{E}}$ |
|---|---|---|---|---|---|---|---|---|---|---|
| $r_{\mathrm{CC}}$ | – | 0.004 | 0.002 | 0.004 | 0.001 | 0.000 | 0.000 | 0.000 | 0.000 | 0.000 |
| $r_{\mathrm{A}_1}$ | | – | 0.000 | 0.000 | 0.000 | 0.000 | 0.000 | 0.000 | 0.000 | 0.000 |
| $\theta_{\mathrm{A}_1}$ | | | – | 0.000 | 0.004 | 0.000 | **0.010** | 0.000 | 0.000 | 0.000 |
| $r_{\mathrm{A}_2}$ | | | | – | 0.000 | 0.000 | 0.000 | 0.000 | 0.000 | 0.000 |
| $\theta_{\mathrm{A}_2}$ | | | | | – | 0.000 | **0.010** | 0.000 | 0.000 | 0.000 |
| $r_{\mathrm{E}}$ | | | | | | – | **0.012** | 0.000 | 0.000 | 0.000 |
| $\theta_{\mathrm{E}}$ | | | | | | | – | 0.000 | 0.000 | 0.000 |
| $\phi_{\mathrm{A}_1}$ | | | | | | | | – | **0.067** | 0.002 |
| $\phi_{\mathrm{A}_2}$ | | | | | | | | | – | 0.002 |
| $\phi_{\mathrm{E}}$ | | | | | | | | | | – |

## B. Analysis of All Interactions of Third and Fourth Order

Finally, the observation reported in the preceding subsection on the two-body interaction information also holds for three- and four-coordinate correlations. Using $n = 10$ generalized coordinates in the present case to describe the full configuration of protonated acetylene, as many as $\binom{10}{3} = 120$ three-coordinate and $\binom{10}{4} = 210$ four-coordinate interaction informations exist. In Fig. 14 the magnitude of all three- and four-coordinate interaction informations, again obtained for classical MD at 600 K and quantum PIMD at 5 K, are plotted in descending order. There are only two (and moreover symmetry-equivalent) significant three-coordinate correlations, namely $I_3(\theta_\mathrm{E}, \phi_\mathrm{E}, \phi_{\mathrm{A}_1})$ and $I_3(\theta_\mathrm{E}, \phi_\mathrm{E}, \phi_{\mathrm{A}_2})$, whereas the follow-up 3-point correlation is already an order of magnitude weaker. Similarly, there is only one significant four-coordinate correlation, namely $I_4(\theta_\mathrm{E}, \phi_\mathrm{E}, \phi_{\mathrm{A}_1}, \phi_{\mathrm{A}_2})$, and all others are much weaker again according to Fig. 14.

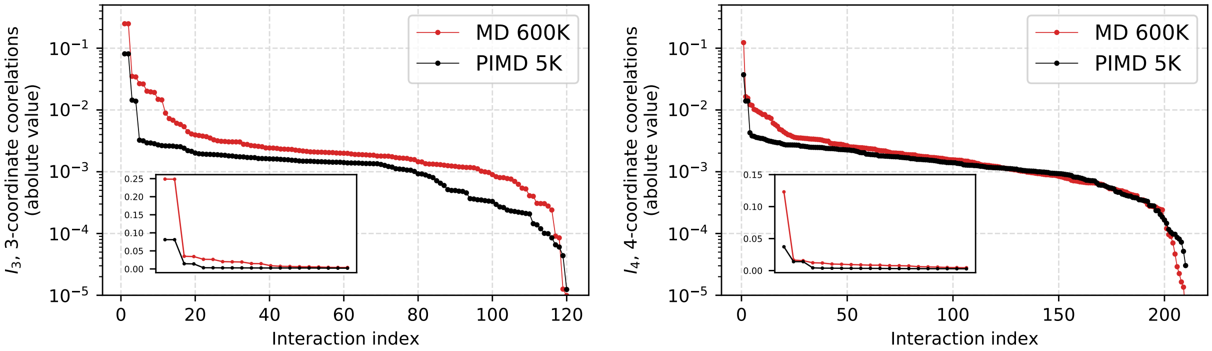


FIG. 14. All three-coordinate (left panel) and four-coordinate (right panel) interaction informations plotted on a logarithmic scale in the order of descending magnitude as obtained from classical MD at 600 K (red) and quantum PIMD at 5 K (black). The respective insets focus on only the 20 strongest $I_3$ and $I_4$ correlations on a linear scale.

## REFERENCES


[1] J. Behler and M. Parrinello, "Generalized neural-network representation of high-dimensional potential-energy surfaces," Phys. Rev. Lett. **98**, 146401 (2007).

[2] J. Behler, "Representing potential energy surfaces by high-dimensional neural network potentials," J. Phys.: Condens. Matter **26**, 183001 (2014).

[3] J. Behler, "Constructing high-dimensional neural network potentials: A tutorial review," Int. J. Quantum Chem. **115**, 1032–1050 (2015).

[4] J. Behler, "First principles neural network potentials for reactive simulations of large molecular and condensed systems," Angew. Chem. Int. Ed. **56**, 12828–12840 (2017).

[5] J. Behler, "Atom-centered symmetry functions for constructing high-dimensional neural network potentials," J. Chem. Phys. **134**, 074106 (2011).

[6] C. Schran, J. Behler, and D. Marx, "Automated Fitting of Neural Network Potentials at Coupled Cluster Accuracy: Protonated Water Clusters as Testing Ground," J. Chem. Theory Comput. **16**, 88–99 (2020).

[7] F. Brieuc, C. Schran, F. Uhl, H. Forbert, and D. Marx, "Converged quantum simulations of reactive solutes in superfluid helium: The Bochum perspective," J. Chem. Phys. **152**, 210901 (2020).

[8] D. Marx and J. Hutter, *Ab Initio Molecular Dynamics: Basic Theory and Advanced Methods* (Cambridge University Press, 2009).

[9] CP2K, released under GPL license; 2019; freely available at `https://www.cp2k.org`.

[10] J. Hutter, M. Iannuzzi, F. Schiffmann, and J. VandeVondele, "cp2k: atomistic simulations of condensed matter systems," Wiley Interdiscip. Rev. Comput. Mol. Sci. **4**, 15–25 (2014).

[11] S. Goedecker, M. Teter, and J. Hutter, "Separable dual-space gaussian pseudopotentials," Phys. Rev. B **54**, 1703–1710 (1996).

[12] F. Brieuc, C. Schran, H. Forbert, and D. Marx, "RubNNet4MD: The RUB Neural Network for Molecular Dynamics Software Package Version 1," (2020), see `https://www.theochem.rub.de/go/rubnnet4md.html`.

[13] S. Shah, F. Palmieri, and M. Datum, "Optimal filtering algorithms for fast learning in feedforward neural networks," Neural Netw. **5**, 779 – 787 (1992).

[14] T. B. Blank and S. D. Brown, "Adaptive, global, extended Kalman filters for training feedforward neural networks," J. Chemom. **8**, 391–407 (1994).

[15] J. B. Witkoskie and D. J. Doren, "Neural network models of potential energy surfaces: Prototypical examples," J. Chem. Theory Comput. **1**, 14–23 (2005).

[16]S. Lorenz, M. Scheffler, and A. Gross, "Descriptions of surface chemical reactions using a neural network representation of the potential-energy surface," Phys. Rev. B **73**, 115431 (2006).

[17]T. B. Adler, G. Knizia, and H.-J. Werner, "A simple and efficient CCSD(T)-F12 approximation," J. Chem. Phys **127**, 221106 (2007).

[18]G. Knizia, T. B. Adler, and H.-J. Werner, "Simplified CCSD(T)-F12 methods: Theory and benchmarks," J. Chem. Phys. **130**, 054104 (2009).

[19]D. E. Woon and T. H. Dunning, "Gaussian basis sets for use in correlated molecular calculations. IV. Calculation of static electrical response properties," J. Chem. Phys. **100**, 2975–2988 (1994).

[20]H. J. Werner, P. J. Knowles, G. Knizia, F. R. Manby, M. Schütz, *et al.*, "MOLPRO, version 2019.1, a package of ab initio programs," (2019), see `https://www.molpro.net`.

[21]F. Brieuc, H. Dammak, and M. Hayoun, "Quantum Thermal Bath for Path Integral Molecular Dynamics Simulation," J. Chem. Theory Comput. **12**, 1351–1359 (2016).

[22]C. Schran, F. Brieuc, and D. Marx, "Converged Colored Noise Path Integral Molecular Dynamics Study of the Zundel Cation Down to Ultralow Temperatures at Coupled Cluster Accuracy," J. Chem. Theory Comput. **14**, 5068–5078 (2018).

[23]M. Ceriotti, M. Parrinello, T. E. Markland, and D. E. Manolopoulos, "Efficient stochastic thermostatting of path integral molecular dynamics," J. Chem. Phys. **133**, 124104 (2010).

[24]L. F. Kozachenko and N. N. Leonenko, "Sample estimate of the entropy of a random vector," Probl. Inf. Transm. **23**, 95–101 (1987).

[25]A. Kraskov, H. Stögbauer, and P. Grassberger, "Estimating mutual information," Phys. Rev. E **69**, 066138 (2004).

[26]V. Hnizdo, E. Darian, A. Fedorowicz, E. Demchuk, S. Li, and H. Singh, "Nearest-neighbor nonparametric method for estimating the configurational entropy of complex molecules," J. Comput. Chem. **28**, 655–668 (2007).

[27]V. Hnizdo, J. Tan, B. J. Killian, and M. K. Gilson, "Efficient calculation of configurational entropy from molecular simulations by combining the mutual-information expansion and nearest-neighbor methods," J. Comput. Chem. **29**, 1605–1614 (2008).

[28]B. Efron and R. Tibshirani, *An Introduction to the Bootstrap* (New York: Chapman & Hall, 1994).
